# Supplementary material for: BALI: Learning Neural Networks via Bayesian Layerwise Inference
Source: arXiv:2411.12102 source file (2024-11-18)
Supplement: Supplementary file 1 [file appendix.tex]

% \section{Layerwise posterior-predictive distribution}

% \begin{align}
% p(\by_{*} | \bx_{*}) &= \int p(\by_{*} | \bx_{*}, \weights) p(\weights | \bX, \by) \mathrm{d} \weights
% \end{align}

% \section{Posterior update with more than 1 weight sample}
% If we draw more than one sample, $\{ \weights_p \}_{p=1}^{P} \sim q_{t}(\weights)$, we treat each corresponding sample $\overleftarrow{\bz}_{n,l,p}$ as an independent pseudo-observation, but we use the tempered (pseudo-)likelihood 
% \begin{equation}
% p( \{ \overleftarrow{\bz}_{n,l,p} \}_{p=1}^{P} | \{ \ba_{n,l,p} \}_{p=1}^{P}, \weights_l) 
% = \prod_{p=1}^{P} p(\bz_{n,l,p} | \ba_{n,l,p}, \weights_l)^{\frac{1}{P}}.
% \end{equation}
% This simplifies computation of the posterior, since the natural parameters are now given by a sum over actual data points and an average over the samples drawn from the previous posterior approximation:
% \begin{align}
% TODO
% \end{align}

% \TODO{Derive formulas for posterior and posterior-predictive of MVBLR model.}
% https://gregorygundersen.com/blog/2020/02/04/bayesian-linear-regression/
